# Supplementary material for: Challenging local realism with human choices
Source: arXiv:1805.04431 source file (2018-11-09)
Supplement: Supplementary file 1 [file SI.tex]

\citation{SackettSP1997}
